# Supplementary material for: Optical coherence of diamond nitrogen-vacancy centers formed by ion implantation and annealing
Source: arXiv:1812.11523 ancillary file (2019-04-23)
Supplement: Supplementary file 1 [file Supplemental_Material.pdf]

# Supplemental Material
# Optical coherence of diamond nitrogen-vacancy centers formed by ion implantation and annealing

S.B. van Dam,[1,2,*] M. Walsh,[3,*] M.J. Degen,[1,2] E. Bersin,[3] S. L. Mouradian,[3,†] A. Galiullin,[1,2] M. Ruf,[1,2] M. IJspeert,[1,2] T. H. Taminiau,[1,2] R. Hanson,[1,2] and D. R. Englund[3]

[1] *QuTech, Delft University of Technology, PO Box 5046, 2600 GA Delft, The Netherlands*
[2] *Kavli Institute of Nanoscience, Delft University of Technology, PO Box 5046, 2600 GA Delft, The Netherlands*
[3] *Department of Electrical Engineering and Computer Science, Massachusetts Institute of Technology, Cambridge, Massachusetts 02139, USA*

## I. SAMPLES AND PROCESSING

### A. Sample A

Sample A and the data-set for sample A were acquired and prepared at MIT. We used a type IIa chemical-vapour-deposition (CVD) grown diamond (Element Six), with a $\langle 100 \rangle$ crystal orientation. The nitrogen content is specified to be less than 5 ppb and is typically less than 1 ppb. The diamond contains a natural abundance of carbon isotopes. This sample was implanted with $^{15}N^{+}$ (minimum purity 98%) at 85 keV (fluence of $10^9$ N/cm$^2$) by Innovion Corporation. After implantation, the diamond underwent cleaning involving a tri-acid clean (boiling sulfuric, nitric and perchloric acids [1:1:1] for one hour) followed by a Piranha clean (sulfuric acid and hydrogen peroxide in a ratio of [3:1]). The sample was subsequently annealed at high temperatures [1]. During the annealing process the temperature was increased at a rate of 1 °C/min and held constant for 2 hours when temperatures reached 400 °C, 800 °C and 1200 °C respectively. The sample underwent the same acid treatment sequence following the annealing process.

### B. Sample B

Sample B was prepared at Delft, with exception of an annealing procedure specified below. The data-set for sample B was acquired at Delft. As with sample A, we used a type IIa CVD grown diamond (Element Six), with a $\langle 100 \rangle$ crystal orientation. The diamond was cut, thinned and polished by Delaware Diamond Knives (DDK) into thin ($\sim$14 $\mu$m) membranes, one of which is sample B. The membrane was implanted with $^{15}N^{+}$ at 400 keV (fluence of $10^8$ N/cm$^2$) by Innovion Corporation. For these ions, the stopping range is approximately 400 nm, as simulated using SRIM [2]. Subsequently, the sample underwent an acid clean in boiling sulfuric, nitric and perchloric acids [1:1:1] for one hour, and 15 minutes in a Piranha solution. Following cleaning, the sample was annealed at high temperatures [1] at Harvard University. During the annealing process the temperature was increased from room temperature to 400 °C over a 4 hours period, and then the temperature was held constant for 8 hours. Subsequently, the temperature was further increased to 800 °C over a 12 hours period, and held constant for 8 hrs. Finally, the temperature was further increased to 1100 °C and held constant for 2 hours. After annealing, the sample underwent the same acid treatments as before annealing. The sample was bonded to a fused silica substrate via Van der Waals forces [3]. The fused silica substrate contains integrated gold MW striplines for spin control as detailed in Ref. [3].

## II. METHODS

### A. Sample A

Experiments were performed using a home-built scanning confocal microscope. The samples were cooled to 4 K using a closed-cycle helium cryostat (Montana Instruments) and were imaged through a 0.9 NA vacuum objective. A Coherent Verdi G5 laser was used to generate 532 nm light and resonant red light tunable around 637 nm was generated by a New Focus Velocity tunable diode laser. Microwave (MW) signals were generated by a Rohde & Schwarz SMIQ06B signal generator and sent through a high-power amplifier (Mini-Circuits ZHL-16W-43+) before delivery to the sample via a wire soldered (15 µm diameter) across the surface. An Excelitas avalanche photodiode (APD) served as our single photon detector. Wavelength/frequency measurements were made with a Princeton Instruments Isoplane SCT 320 spectrometer and/or a WS7 HighFinesse wavelength meter (these two devices were calibrated relative to each other by scanning the Velocity laser through the wavelengths of interest). All digital signals used to produce pulse sequences were generated on a PulseBlaster ESR-Pro from SpinCore; additional analog control and photon counting were performed on a USB NI6343 from National Instruments. The automated measurement sequence for

* These authors contributed equally.
† Present Address: Department of Physics, University of California Berkeley, California 94720, USA

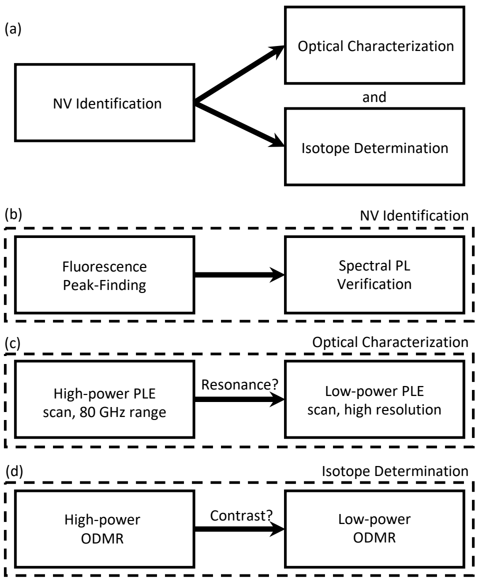


FIG. S1. **Measurement sequence for sample A. (a)** The three parts of the experimental sequence: NV identification, optical characterization and isotope recognition are executed by an automated protocol. **(b)** Fluorescent peaks are identified after processing the image with a spatial band-pass filter and taking peaks above a certain threshold (more detail in the text). This yields many NV candidates that are tested for the presence of PL between 636-639 nm using a spectrometer to confirm the peak is from an NV. **(c)** Using the wavelength of the peak identified in **(b)**, we coarsely tune the resonant laser to the emitter and scan over the entire range allowed by the cavity (82 GHz) with high power to assure we do not miss the transition peak. Once found, we repeat the measurement with higher resolution and low enough power to avoid power-broadening. **(d)** For each NV center a low-power continuous wave (CW) ODMR spectrum is taken, to find the N isotope.

sample A is shown in Figure S1 in detail.

### 1. *NV identification*

Fluorescent spots were identified using a peak-detection algorithm on a confocal scan. The image was first filtered using a spatial band-pass filter (constructed with a "low-pass" Gaussian kernel with a full-width at half-maximum (FWHM) of 235 nm and a "high-pass" Gaussian kernel with a spatial FWHM of 700 nm). A peak is defined as a pixel that is greater than or equal to its 4 nearest neighbors and greater than the 4 second nearest neighbors. A threshold was calculated to be 1-2 standard deviations above the median pixel value. Only peaks that carried an intensity value above the calculated threshold were used in the experiment. Each image was inspected, and the threshold fine-tuned before continuing the experiment to ensure that every visible peak was located.

The fluorescent spots were validated by examining a PL spectrum under 532 nm excitation for a peak between 636 nm and 639 nm (the range in which we can tune our resonant laser). No peaks were found out of this range. We illuminated the sample with 300 µW of power while the spectrometer acquired a measurement with an exposure of 10 seconds (a relatively short amount of time compared to the optical characterization). Peaks were detected after noise removal using a similar technique as described above for the fluorescent spot detection.

### 2. *Optical characterization*

All photoluminescence excitation (PLE) measurements in this section will refer to a pulse sequence described in Figure 2c of the main text. The duration of the green repump was 2 µs with a power of about 300 µW. The collection bin was 10 µs with 3 µW of resonant illumination power that could be attenuated with optical-density (OD) filters. The frequency of the excitation was monitored continuously using the wavelength meter.

The first step in optical characterization was a PLE scan at high power (no attenuation with OD filters). For each ZPL peak identified, the laser was coarsely tuned to the ZPL frequency, then tuned across the full range of the Velocity laser's external cavity range (82 GHz) with a resolution of 275 MHz. This sequence was averaged $10^4$ times at each frequency to ensure that the SNR is large enough to find an NV signal (Table S1 shows the statistics corresponding to optical and isotope recognition of our NV set).

The automated protocol roughly identified statistically relevant peaks (nearly all locations that were NVs revealed two such peaks; one for $E_x$ and $E_y$). A sum of Gaussian lineshapes were fit to the data-set based on the number of peaks detected. The location and width of the peak were all recorded for use in the high-resolution scans.

Next, the high-resolution scans were performed using a low power red excitation (300 nW, obtained with an OD filter) to avoid power-broadening. To account for the lower excitation power, we performed $10^6$ averages. The scan range and resolution were determined by the location and width of the previous high-power scan.

Gaussian lineshapes were fit to the final low-power, high-resolution scans in the same manner as for the high-power scans. The center ZPL position is midway between the $E_x$ and $E_y$ transitions, and the splitting is half the distance between them.

### 3. *Isotope recognition*

The final step in the measurement protocol is to measure a continuous-wave (CW) optically-detected magnetic resonance (ODMR) that probes the NV fine structure. We determined the emitter's orientation by sweeping a strong MW field over each of the 4 possible orien-

| | no ODMR contrast | no resolvable hyperfine | hyperfine resolved | failed | |
|---|---|---|---|---|---|
| PLE signal | 59 | 14 | 36 | 1 | **110** |
| no PLE signal | 5 | 2 | 0 | 3 | **10** |
| | **64** | **16** | **36** | **4** | **120** |

TABLE S1. **Table summarizing all data for sample A.** This table has the numeric breakdown of all NVs reported. The bold numbers indicate a particular column or row summation. NVs that resulted in an error were either due to a hardware failure during the automated protocol or a peak that was detected in one scan but could not be found again (likely due to a false-positive originally).

tations (pre-characterized prior to each run). Once determined, we iteratively lowered the MW power until the ODMR signal had resolvable hyperfine transitions (up to 10 dB lower than the power used to determine the orientation). The NV isotope was determined by inspection of the multiplicity of the number of dips in the ODMR spectrum.

Almost half of the NVs identified (showing both PLE and ODMR signals) had unidentifiable ODMR spectra. Figure S2 shows a summary of all identified emitters. It is important to note that the distribution of both categorized ($^{14}$NV and $^{15}$NV) and un-categorized NVs follow the same distribution (as seen by the overlapping CDF in Figure S2a and the same shape of histograms in Figure S2b-c).

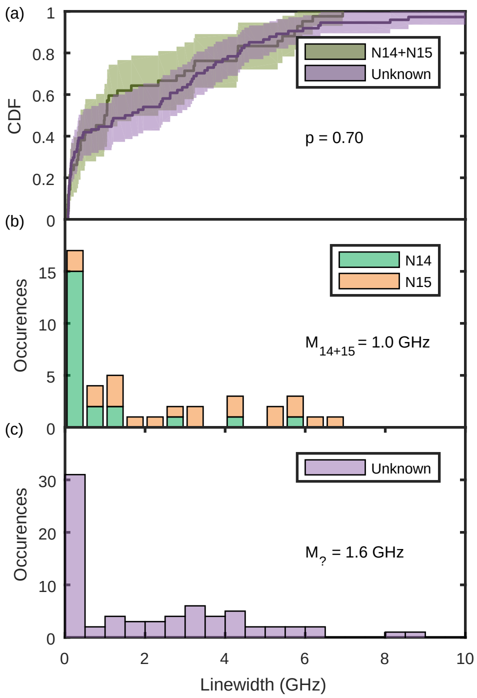


FIG. S2. **Summary of all data for sample A. (a)** A CDF representing the distributions of unknown isotope to known isotope ZPL linewidths. A similar shape indicates that both sample sets are drawn from the same distribution indicating there is no inherent bias towards sampling $^{14}$NV or $^{15}$NV. The probability to obtain these results if the samples are drawn from the same distribution (p) is evaluated by a Wilcoxon rank-sum test. **(b)** A stacked histogram showing the all $^{14}$NV and $^{15}$NV ZPL linewidths. The median linewidth (M) is indicated. **(c)** A histogram showing the linewidths for the set of ZPLs with an unknown host isotope.

## B. Sample B

Sample B is maintained at a temperature of 4 K in a closed-cycle cryostation (Montana Instruments). The optical and electronic elements of the experimental setup are as previously described in Ref. [4]. We describe the measurement sequence for sample B, schematically presented in Figure S3, in detail.

### 1. *NV identification*

Fluorescent spots were identified by inspection of a confocal scan. On these spots a spatial optimization in three dimensions was performed. The automated protocol proceeded if the spot could be fit with a Gaussian shape. Next, a CW ODMR measurement was performed at high microwave power. The high power was used to maximize the visibility of an ODMR dip. The dip was fit with a Gaussian curve to find the resonance frequency that was used in the remainder of the protocol for microwave driving.

If spatial optimization was successful and an ODMR dip observed, a spot was marked as an NV center. Out of 52 spots identified as an NV center following this protocol, five contained two NV centers. Because a unique link between ODMR for isotope-recognition and the optical linewidth was not made, these NVs were left out of the final analysis. NVs with both narrow and broad optical linewidths were identified in these five spots, as well as at least one $^{14}$NV.

### 2. *Optical characterization*

In this section we detail the optical characterization for sample B as described in Figure 2c-d of the main text.

The first step in optical characterization was a PLE scan at high power, with red and green excitation interleaved for each step. We applied 100 nW of red power (measured before the objective) for 100 µs, followed by 100 µW green power for 10 µs and a 10 µs wait time. This sequence was repeated for a total integration time of 10 ms for each data point. The scan was carried out over a range of 500 GHz, with a resolution of approxi-

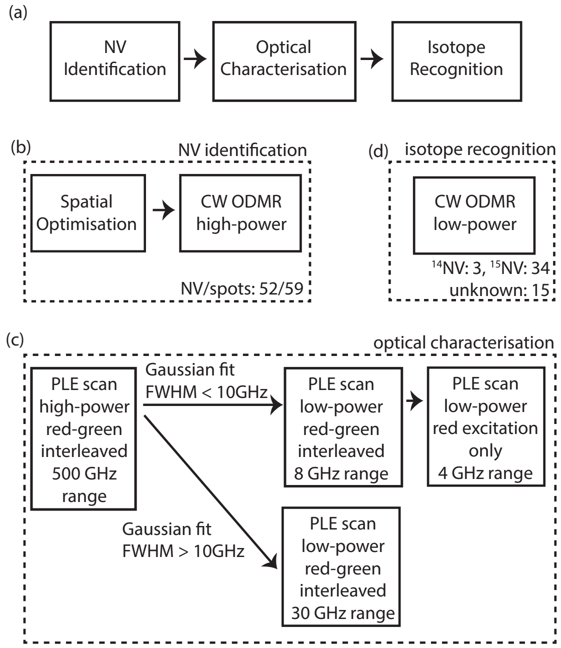


FIG. S3. **Measurement sequence for sample B. (a)** The three parts of the experimental sequence: NV identification, optical characterization and isotope recognition are executed by an automated protocol. **(b)** Out of a total of 64 fluorescent spots at the implantation depth and deeper in the sample, 57 were identified as NV centers, based on a Gaussian spatial profile and the presence of an ODMR dip. 52 of these spots contained single NV centers **(c)** After a broad range scan to determine the position of the optical resonances, separate sequences are performed for very broad linewidths ($>$ 10 GHz) and the other linewidths, to restrict measurement time. Measurements probing the linewidth free from spectral diffusion (refered to as low-power red excitation only) are performed only if the linewidth was not very broad. **(d)** For each NV center a low-power CW ODMR spectrum is taken, to find the N isotope.

mately 10 MHz.

The laser wavelength was monitored after each laser frequency step using a wavelength meter. During all optical scans microwave driving was applied to observe optical lines for all spin projections in the red-green interleaved scan, and to prevent optical pumping in the scans probing short-timescale dynamics.

Automated protocols were used to fit a Gaussian lineshape to the peaks, determining the location of the two highest peaks. The center ZPL position is midway between the highest peaks, and the strain splitting is the half distance. For four NVs no optical resonances were found in the 500 GHz range scanned in the automated protocol (between 470.3 THz and 470.8 THz). For three of these, optical resonances were found manually outside this range (around 469.7 THz, 470.2 THz, and 471.1 THz). For one NV no optical lines were found in a range from 469.4 THz to 471.4 THz.

We continued with scans around the resonances, using a low power red excitation (12 nW) to avoid any power-broadening. To restrict measurement time, the performed measurements depend on the fitted linewidth in the large-range scan as follows.

If the fitted linewidth in the broad-range scan was very broad ($>$ 10 GHz), a PLE scan with interleaved red and green was subsequently carried out over a range of approximately 30 GHz. The resolution of this scan was 30 MHz. The timing of the sequence is as described for the broad-range scan.

If the fitted linewidth was $<$ 10 GHz, we performed a single PLE scan interleaving red and green excitation for each data point over a range of 8 GHz (resolution 4 MHz, same timings as the broad-range scan). Next, we proceeded with 30 scans with red excitation, with repumping only in between each scan. The range of these scans was 4 GHz, with a resolution of approximately 4 MHz. The integration time for each pixel was 20 ms, and the total scan time over the full 4 GHz range was approximately 40 seconds. After each scan we performed a second scan over the resonance to determine if the NV ionized during the original scan. We fit a Lorentzian to the non-ionized traces, and extract the FWHM, $\bar{\gamma}$, from their weighted average:

$$\bar{\gamma} = \frac{\sum_i \gamma_i \sigma_i^{-2}}{\sum_i \sigma_i^{-2}}, \tag{1}$$

where $\gamma_i$ are the fitted FWHM of the individual traces, and $\sigma_i$ the corresponding standard error of the fit parameter.

### 3. *Isotope recognition*

The final step in the measurement protocol was an ODMR measurement probing the NV fine structure, scanning around the resonance detected during the NV identification (step 1). This ODMR measurement was performed at 7 dB attenuation relative to the ODMR measurement during NV characterization, to avoid power-broadening. The NV isotope was determined by inspection of the multiplicity of the number of dips in the ODMR spectrum, and confirmed by the best goodness of fit out of fits with Gaussian dips with hyperfine splittings fixed to the $^{14}$NV or $^{15}$NV values. The isotope could not be reliably identified by inspection in 15 NV centers located at the implantation depth. We note that these contained both NV centers with broad ($>$ 500 MHz, 13 NVs) and narrow ($<$ 500 MHz, 2 NVs) linewidths.

Table S2 shows a summary of the PLE and ODMR contrast for spots at the implantation depth and deeper in the diamond. In S4 a summary of the optical linewidths is shown, including the NVs with unknown isotopes. Similar to the observations for sample A, we find that the cumulative density function for the unknown isotopes and the combined $^{14}$NV and $^{15}$NV data overlap.

| | PLE signal | no PLE signal | |
|---|---|---|---|
| ODMR isotope resolvable | 35 | 0 | **35** |
| ODMR isotope unresolvable | 16 | 1 | **17** |
| no ODMR contrast | 1 | 4 | **5** |
| | **51** | **5** | **57** |

TABLE S2. **Table summarizing all data for sample B.** This table has the numeric breakdown of all fluorescent spots reported, at the implantation depth (52 spots) and deeper in the diamond (5 NVs). Not included are two data-points for which spatial optimization was not successful, and 5 spots that contained more than one NV. The bold numbers indicate a particular column or row summation.

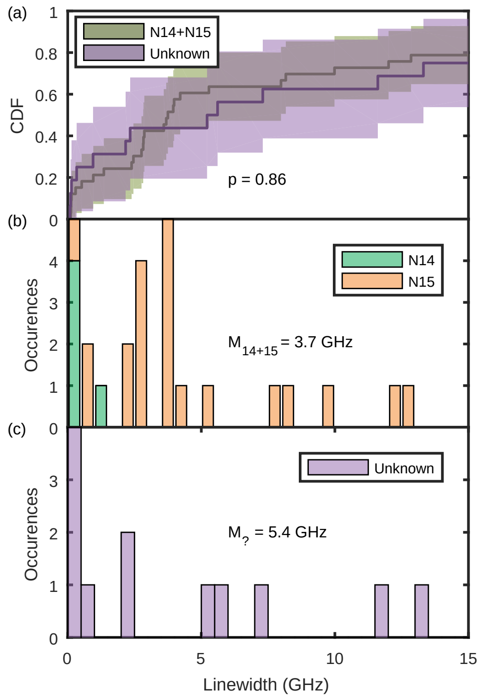


FIG. S4. **Summary of all data for sample B. (a)** A CDF representing the distributions of unknown isotope to known isotope ZPL linewidths. A similar shape indicates that both sample sets are drawn from the same distribution indicating there is no inherent bias towards sampling $^{14}$NV or $^{15}$NV. The probability to obtain these results if the samples are drawn from the same distribution (p) is evaluated by a Wilcoxon rank-sum test. **(b)** A stacked histogram showing the all $^{14}$NV and $^{15}$NV ZPL linewidths. The median linewidth (M) is indicated. **(c)** A histogram showing the linewidths for the set of ZPLs with an unknown host isotope. The histograms in **(c)** and **(d)** do not show data for 7 $^{15}$NV and 4 NVs with unknown isotope as they are out of the range (> 15 GHz).

## III. CHARACTERIZATION OF REPUMP LASER-INDUCED SPECTRAL DIFFUSION

On sample B we performed scans to isolate short timescale fluctuations from repump laser-induced spectral diffusion (Figure 2(d) of the main text).

For each NV center we performed 30 consecutive scans, with a green repump laser pulse applied only in between the scans. The scans in which the NV center did not ionize are selected. We fit a Lorentzian curve to the resonance in each scan and calculate the weighted average for each NV center (see Eq. 1). We also fit the sum of the scans with a Gaussian curve, extracting the FWHM including repump laser-induced spectral diffusion. When correlating the two analyses, as shown in Figure S5, we find that the Lorentzian linewidths are mostly less than 200 MHz, while further broadening in the linewidth can be attributed to laser-induced spectral diffusion.

Protocols using resonant charge repumping [5] and real-time monitoring of the transition frequency [6] have been used to reduce linewidths broadened to <200 MHz by slow spectral diffusion. However, for larger broadening, and especially for the very broad (>1 GHz) linewidths for $^{15}$NVs, such a repump scheme is challenging as after each remaining frequency jump the resonances shift significantly, complicating the locating of the new resonances within an acceptable time.

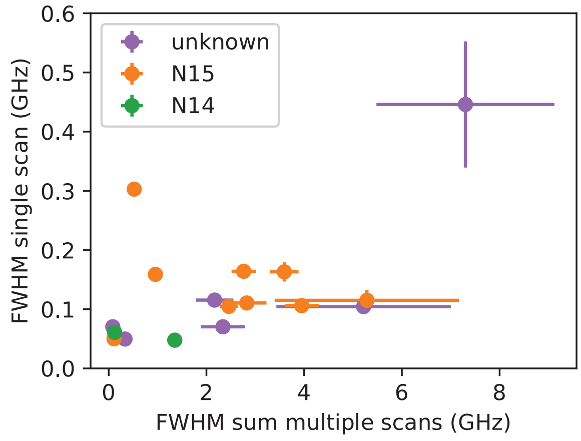


FIG. S5. **Optical linewidths from scans with red excitation only.** Consecutive scans over a single resonance are performed as described in the text. The FWHM of the optical linewidth in individual scans ($y$-axis) is correlated to the FWHM of the summed scans including repump laser-induced spectral diffusion ($x$-axis). We conclude that the Lorentzian linewidths are mostly less than 200 MHz, while further broadening in the linewidth can be attributed to laser-induced spectral diffusion. This figure contains data for NV centers at the implantation depth with linewidths < 10 GHz (Figure S3).

## IV. NV DENSITIES

In sample A (see confocal scans in Figure 2a of the main text), the NV areal densities estimated from the verified isotopes at the implantation depth are at least $3.9\times10^{-2}$ $^{14}$NVs/µm$^2$ and $3.5\times10^{-2}$ $^{15}$NVs/µm$^2$. When assuming that the isotope distribution over the NVs with unknown isotope follows the same distribution as for the known NVs (this assumption is supported by the overlapping linewidth distributions in Figure S2), the areal density estimates are $5.1\times10^{-2}$ $^{14}$NVs/µm$^2$ and $4.7\times10^{-2}$ $^{15}$NVs/µm$^2$. This corresponds to a conversion efficiency of implanted $^{15}$N to NV of approximately 3.5%-4.7%.

At a scan deeper in the sample over the same area (Figure 2a, inset) we found 3 NVs, that we assume to be $^{14}$NV given their location in the diamond well below the implantation depth. The native areal density of $^{14}$NVs that we estimate from this is $3\times10^{-2}$ $^{14}$NVs/µm$^2$.

Confocal scans of sample B are shown in Figure S6, at the implantation depth and deeper into the sample to illustrate the change in NV density due to implantation.

The confocal scan at the implantation depth ($\sim$ 400 nm, Figure S6a) displays around $\sim$ 180 fluorescent spots. We characterized 59 of these spots from the highlighted region in Figure S6a, identifying 57 NV centers (47 single NVs in a confocal spot and 5 spots with two NVs). We are able to determine the isotope for 37 NVs, 3 out of which are $^{14}$NVs, and 34 are $^{15}$NVs. From this, a lower-bound estimate of the $^{14}$NV areal density after implantation is $4\times10^{-2}$ $^{14}$NVs/µm$^2$. We estimate the $^{15}$NV areal density to be at least $5\times10^{-1}$ $^{15}$NVs/µm$^2$. When assuming that the unknown isotopes follow the distribution of isotopes for the known isotopes (as for sample A, this is supported by the overlapping linewidth distributions in Figure S4), the areal density estimates are $6\times10^{-2}$ $^{14}$NVs/µm$^2$ and $7\times10^{-1}$ $^{15}$NVs/µm$^2$. This corresponds to an estimated conversion efficiency of implanted $^{15}$N to NV of approximately 50%-70%. We attribute differences in conversion efficiencies between sample A and sample B to the difference in implantation parameters [7].

We characterized 5 out of 6 bright fluorescent spots in the deep scan ($\approx$ 5 $\mu$m depth, Figure S6 **b**). All 5 spots were identified as NVs, and all displayed narrow linewidths in the red-green interleaved scan. The isotope were found to be $^{14}$N for 3 out of 5 NVs, whereas the isotope could not be reliably determined from the ODMR measurement for 2 NVs (this is a comparable ratio of known versus undetermined isotopes as at the implantation depth). Because their location in the diamond was well below the implantation depth, these findings strongly suggest that these fluorescent spots are naturally occurring $^{14}$NV. A best estimate of the $^{14}$NV areal density before implantation is therefore $3\times10^{-2}$ $^{14}$NVs/µm$^2$.

Although the sample sizes are small, comparing the estimated $^{14}$NV densities at the implantation depth and deeper in the diamond we find indications that $^{14}$NVs at the implantation depth are created during implantation in both sample A and B.

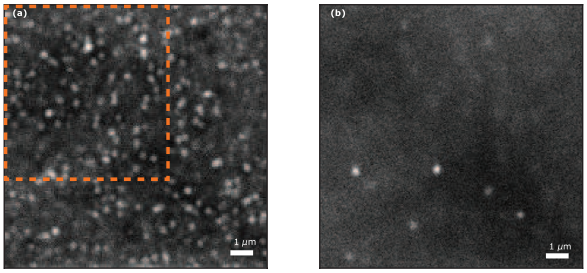


FIG. S6. **Confocal scans of sample B (a)** at the implantation depth and **(b)** at ≈5 µm under the diamond surface. The orange box indicates the approximate region at the implantation depth in which fluorescent spots were characterized.


[1] Y. Chu, N. P. de Leon, B. J. Shields, B. Hausmann, R. Evans, E. Togan, M. J. Burek, M. Markham, A. Stacey, A. S. Zibrov, A. Yacoby, D. J. Twitchen, M. Lončar, H. Park, P. Maletinsky, and M. D. Lukin, Nano Lett. **14**, 1982 (2014).

[2] J. F. Ziegler, M. Ziegler, and J. Biersack, The Stopping and Range of Ions in Matter (SRIM-2013, http://www.srim.org/).

[3] S. Bogdanovic, M. S. Z. Liddy, S. B. van Dam, L. C. Coenen, T. Fink, M. Loncar, and R. Hanson, APL photonics **2**, 126101 (2017).

[4] M. S. Blok, C. Bonato, M. L. Markham, D. J. Twitchen, V. V. Dobrovitski, and R. Hanson, Nat. Phys. **10**, 189 (2014).

[5] P. Siyushev, H. Pinto, M. Vörös, A. Gali, F. Jelezko, and J. Wrachtrup, Phys. Rev. Lett. **110**, 167402 (2013).

[6] B. Hensen, H. Bernien, A. E. Dréau, A. Reiserer, N. Kalb, M. S. Blok, J. Ruitenberg, R. F. L. Vermeulen, R. N. Schouten, C. Abellán, W. Amaya, V. Pruneri, M. W. Mitchell, M. Markham, D. J. Twitchen, D. Elkouss, S. Wehner, T. H. Taminiau, and R. Hanson, Nature **526**, 682 (2015).

[7] S. Pezzagna, B. Naydenov, F. Jelezko, J. Wrachtrup, and J. Meijer, New J. Phys. **12**, 065017 (2010).
